# Supplementary material for: Re-evaluating Evaluation in Text Summarization
Source: arXiv:2010.07100 source file (2020-10-14)
Supplement: Supplementary file 1 [file appendix.tex]

\section{Appendices}
\label{sec:appendix}
\subsection{Sampling and Scoring Methodology}
\begin{algorithm}[h!]
\caption{\label{alg:sampling}Sampling Methodology}
\small
\SetAlgoLined
\KwData{$(d_i, r_i, S_i) \in D$\\
where $D$ is \texttt{CNNDM} test set, $d_i$ is source document, $r_i$ is reference summary, and $S_i$ is a set of individual system summaries $s_{ij} \in S_i$.\\

$M$ = [ROUGE-1, ROUGE-2, ROUGE-L, BertScore, MoverScore]
}
\KwOutput{$D_{out}$: sampled set of documents}
$\mu_{m, i} := mean(\{m(r_i, s_{ij}) \forall s_{ij} \in S_i\})$, $m \in M$ \\
$\sigma_{m, i} := std.dev(\{m(r_i, s_{ij}) \forall s_{ij} \in S_i\})$, $m \in M$ \\
$D_{out} := \{\}$ \\ 
$n_1 := |D| / 5$ \\

\For{$m \in M$}{ \\
$D'$ := $[d_i: d_i \in D]$ sorted by  $\mu_{m,i}$ \\
    \For{$k \in [0, 1, 2, 3, 4]$}{
        $D'_k = D'[i*n_1: (i+1)*n_1]$ \\
        $D''_k = [d_i: d_i \in D'_k]$ sorted by $\sigma_{m,i}$
        $n_2 = |D''_k| / 4$ \\
        \For{$l \in [0, 1, 2, 3]$}{
            $D''_{kl} = D''_k[l*n_2 : (l+1)*n_2]$ \\
            Randomly sample $d_i$ from $D''_{kl}$ \\
            $D_{out} = D_{out} \cup {d_i}$
        }
    }
}
\end{algorithm}

\subsection{Observations on \texttt{TAC-2009} dataset}
\label{sec:tac_2009_obs}
\begin{figure}[ht]
  \centering
  \subfloat[TAC-2009 topk]{
    \label{fig:tac_9_topk}
    \includegraphics[width=0.50\linewidth]{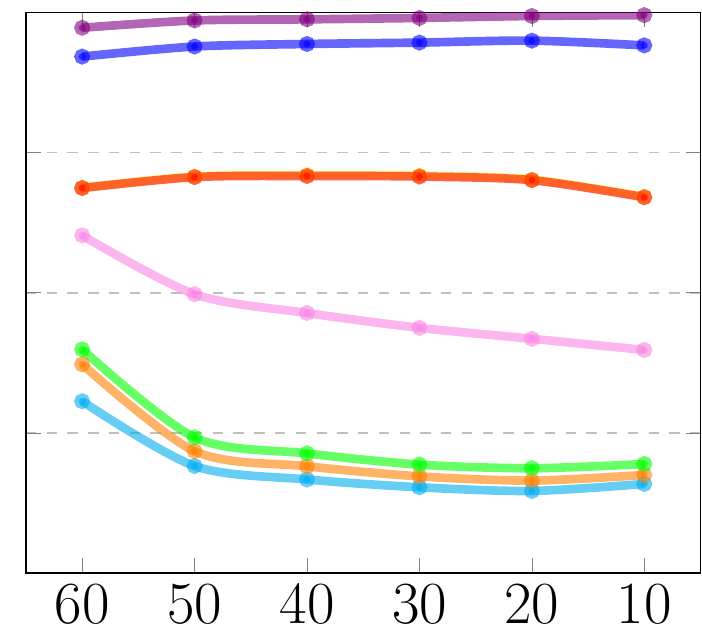}
  }
  \subfloat[TAC-2009 different quality systems.]{
    \label{fig:tac_9_lmh}
    \includegraphics[width=0.48\linewidth]{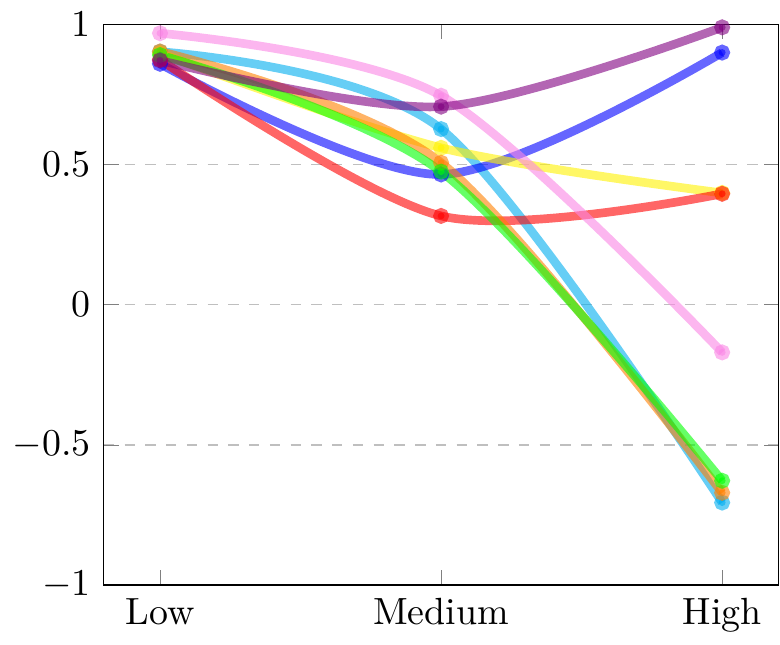}
  }
  \caption{\label{fig:tac_9_sys_level}Results of Sec. \ref{sec:topk_human} and \ref{sec:quality_human}}
\end{figure}

\begin{figure}[h!]
    \centering
    \includegraphics[width=0.7\linewidth]{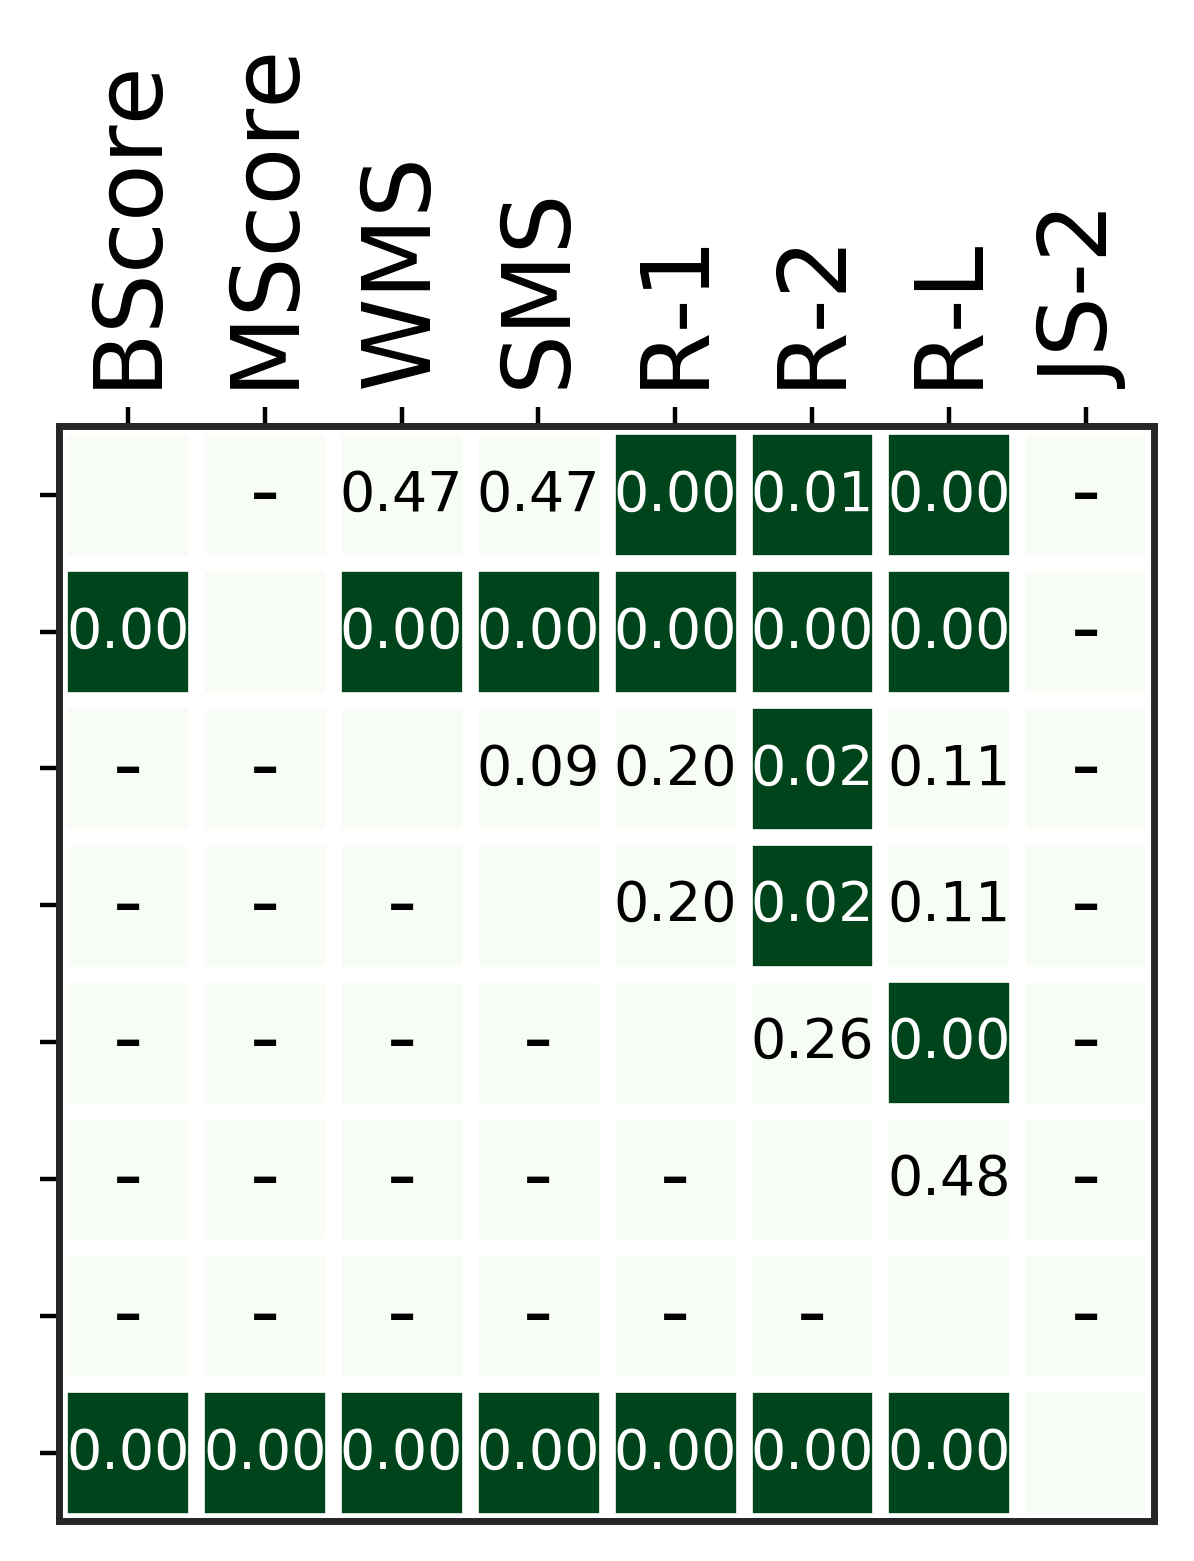}
    \caption{\label{fig:tac09_williams}Results of Section \ref{sec:williams_test}}
\end{figure}

\subsection{Pearson's Correlation For William's test}
\label{sec:williams_pearson}
\begin{figure}[h!]
    \centering
    \includegraphics[width=\linewidth]{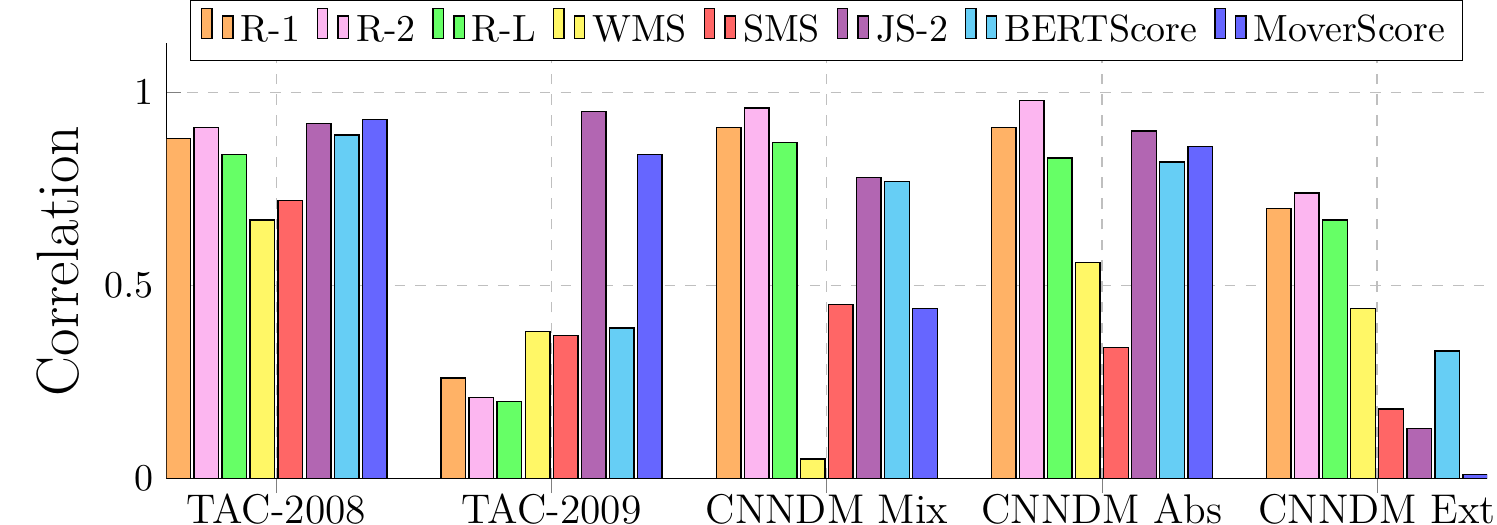}
    \caption{\label{fig:williams_pearson}Pearson Correlations of William's test.}
\end{figure}

\section{Supplemental Material}
\label{sec:supplemental}
